# Supplementary material for: DPLM-2: A Multimodal Diffusion Protein Language Model
Source: arXiv:2410.13782 source file (2024-10-17)
Supplement: Supplementary file 1 [file 100_appendix.tex]

\section{Reparameterizaed Discrete Diffusion Models (RDM)}
\label{app: rdm}
\method uses reparameterized discrete diffusion model (RDM) as its discrete diffusion framework~\citep{zheng2023reparameterized}.
Here we briefly summarize its basic training and sampling. Please refer to~\citet{zheng2023reparameterized} for more details.

\citet{zheng2023reparameterized} shows that the backward transition of discrete diffusion models $q(\bm{x}_{t-1}|\bm{x}_t, \bm{x}_0)$ can be rewritten as 
\begin{align}
   & q(\bm{x}_{t-1}|\bm{x}_t, \bm{x}_0) \nonumber \\
    &= \begin{cases}
\texttt{Cat}\left(\bm{x}_{t-1};\lambda_{t-1}^{(1)}\bm{x}_t + (1-\lambda_{t-1}^{(1)})\bm{q}_{\text{noise}}\right), \text{if } \bm{x}_t=\bm{x}_0 \nonumber \\
\texttt{Cat}\left(\bm{x}_{t-1};\lambda_{t-1}^{(2)}\bm{x}_t + (1-\lambda_{t-1}^{(2)})\bm{q}_{\text{noise}}(\bm{x}_t)\right), \text{if } \bm{x}_t \not=\bm{x}_0
\end{cases}
\label{eqn: backward transition}
\end{align}
where $\bm{q}_{\text{noise}}(\bm{x}_t) = \beta_t\bm{x}_t + (1-\beta_t)\bm{q}_{\text{noise}}$, and both $\lambda_{t-1}^{(1)}$ and $\lambda_{t-1}^{(2)}$ are constants relating to $\beta_t$ and $\beta_{t-1}$. This reformulation interprets the backward transition as a mixture distribution. Sampling from it is equivalent to first sampling from a Bernoulli distribution and then the corresponding component distribution, \ie,
$$
\begin{aligned}
v_{t-1}^{(1)}\sim \text{Bernoulli}\left(\lambda_{t-1}^{(1)}\right),&&
\bm{u}_t^{(1)}\sim \texttt{Cat}\left(\bm{u}; \bm{p}=\bm{q}_{\text{noise}}\right),&\\
v_{t-1}^{(2)}\sim \text{Bernoulli}\left(\lambda_{t-1}^{(2)}\right),&& 
\bm{u}_t^{(2)}\sim \texttt{Cat}\left(\bm{u}; \bm{p}=\bm{q}_{\text{noise}}(\bm{x}_t) \right),&
\end{aligned}\\
$$
$$
\bm{x}_{t-1}=\left\{
\begin{aligned}
v_{t-1}^{(1)}\bm{x}_t + \left(1-v_{t-1}^{(1)}\right)\bm{u}_t^{(1)},&&\text{if }\bm{x}_t=\bm{x}_0\\
v_{t-1}^{(2)}\bm{x}_t + \left(1-v_{t-1}^{(2)}\right)\bm{u}_t^{(2)},&&\text{if }\bm{x}_t\not=\bm{x}_0
\end{aligned}
\right..
$$
This reparameterizes the transitions into $q(\bm{x}_t, \bm{v}_{t-1}|\bm{x}_t, \bm{x}_0)$ and $p_{\bm{\theta}}(\bm{x}_{t-1}, \bm{v}_{t-1}|\bm{x}_t)$. 
With this reparameterization, the training objective of diffusion models (\ie, the variational bound of negative log-likelihood) becomes
\begin{align}
& -\mathbb{E}_q(\bm{x}_{1:T}, \bm{v}_{1:T}|\bm{x}_0)\left[\log \frac{p_\theta(\bm{x}_0,\bm{x}_{1:T},\bm{v}_{1:T})}{q(\bm{x}_{1:T},\bm{v}_{1:T}|\bm{x}_0)} \right] \nonumber \\
& =L_1 + \sum_{t=2}^T L_t + \text{const.}, \nonumber
\end{align}
where $L_1=-\mathbb{E}_{q(\bm{x}_1|\bm{x}_0)}\left[\log p_\theta(\bm{x}_0|\bm{x}_1)\right]$ and \citet{zheng2023reparameterized} shows that $L_t$ can be simplified into
% \begin{equation}
% L_t = \mathbb{E}\left[-\lambda_{t-1}^{(2)}\left(1-\mathds{1}(\bm{x}_t=\bm{x}_0)\right)\log p_{\bm{\theta}}(\bm{x}_0|\bm{x}_t)\right], 
% \label{eqn: reparam objective}
% \end{equation}
% where $\mathds{1}(\cdot)$ is indicator function. This is exactly a weighted cross-entropy loss on the perturbed data, \aka the masked language modeling objective~\citep{devlin2019bert}.
Notably, training with different noise schedules only differs in the weighting of the objective.

During sampling, RDM leverages this observation and proposes to employ a discriminative approach.
Specifically, it denoises a token only when it receives a top-$k$ score (log-probability) from the network where $k$ in each step is determined by a denoising schedule. The overall sampling process is shown in algorithm \ref{alg:rdm:sampling}.

\begin{algorithm}[H] %
   \caption{Sampling from RDM}
   \label{alg:rdm:sampling}
    \begin{algorithmic}
    \State {\bfseries Input:} trained network $f_\theta\left(\cdot\right)$ and temperature $\tau$.
    \State {\bfseries Output:} generated sample $\xt{0}$.
    \For{$n = 1,2,\dots,N$}
        \State Initialize $\bm{x}_{T,n} \sim q_{\text{noise}}$;
        \State Initialize $b_{T,n} = 0$;
    \EndFor
    \For{$t = T,\dots,1$}
        \For{$n = 1,2,\dots,N$}
            \State Draw $\widetilde{\bm{x}}_{0,n} \sim \operatorname{Categorical}\left(f_\theta\left(\bm{x}_{t,n}\right)\!/\tau\right)$;
            \State Generate $\bm{v}_{t-1,n}$ according to $\log p(\widetilde{\bm{x}}_{0,n})$
            \If{$b_{t,n} = 1$}
            \State Draw $\bm{u}_{t,n}^{(1)} \sim q_\text{noise}$;
            \State $\bm{x}_{t-1,n} = v_{t-1,n}^{(1)}\bm{x}_{t,n} + \left(1-v_{t-1,n}^{(1)}\right)\bm{u}_{t,n}^{(1)}$;
            \Else
            \State Draw $\bm{u}_{t,n}^{(2)} \sim q_\text{noise}(\bm{x}_{t,n})$;
            \State $\bm{x}_{t-1,n} = v_{t-1,n}^{(2)}\widetilde{\bm{x}}_{0,n} + \left(1-v_{t-1,n}^{(2)}\right)\bm{x}_{t,n}^{(2)}$;
            \EndIf
            \State Let $b_{t-1,n} = b_{t,n} \land v_{t-1,n}^{(1)} \lor v_{t-1,n}^{(2)}$;
        \EndFor
    \EndFor
    \State {\bfseries Return} $\bm{x}_{0,1:N}$.
    \end{algorithmic}
\end{algorithm}

\section{Additional Experimental Details}
% Discussion on the two-stage pretraining details: why we use two-stage pretraining, the performance of two-stage pretraining, comparision of official ESM2 and the one pretrained by us.

\subsection{Pre-training of \method}
During the training phase, we investigate two different approaches: (1) training with the diffusion objective from scratch, and (2) what we refer to as two-stage training, which consists of initial training with the masked language modeling (MLM) objective followed by continuous training with the diffusion objective.

\paragraph{Empirical Observation:} In our preliminary experiments, we observed that discrete diffusion pre-training "from scratch (FS)" often yielded instability in the form of frequent loss spiking, therefore hurting our model performance.
% We find that training \method from scratch is a bit challenging and converges slowly. 

\paragraph{Our Hypothesis:} We noticed that the absorbing diffusion objective leads to a variable masking ratio ranging from 0\% to 100\%, while conventional MLM objective's masking ratio keep fixed at 15\% such that a masked LM is always exposed to rich condition of 85\% observation/context. 
In other words, in contrast to MLM, for absorbing discrete diffusion models like DPLM, in some of the extreme cases there are nearly all tokens getting masked, which means that the model is required to recover all tokens of the ground-truth sequence from nothing). 
This could impose severe learning challenges, especially at the early phase of pre-training, where the model has yet not acquired sufficient capability to extract informative features and correlations from limited observation.
% Training with MLM first allows the model to get a better starting point, and then get the final model through diffusion adaptation, sharing similar idea as~\citet{ye2023diffusion}. 

\paragraph{Solution in Principle:}  Inspired by the success of curriculum learning in non-autoregressive text generation [1,2,3,4,5], we suggested that a masking warmup strategy could mitigate this issue, where we can start with a small upper bound of masking ratio (e.g., 15\% as conventional MLM, to preserve a high proportion of observation) in the early phase of pre-training, and then gradually increase the masking ratio towards the authentic discrete diffusion objective during pre-training.
% This kind of strategy similar to curriculum learning makes the training effect better.

\paragraph{Solution in Practice:} 
In the current form of our manuscript, adhering to this principle, we used a two-stage training method: initialized DPLM from an established masked LM, either from our in-house pre-trained one or from the official ESM-2 checkpoint, and then trained DPLM by the discrete diffusion language modeling objective afterwards. Though it may or may not lead to the best model performance, it offers the possibilities of standing on the shoulders of any pre-trained masked LM such as ESM2 or the advanced LM architecture such as a Llama/Mistral-style masked LMs, in the broad open-source AI community. This also enables us to bypass the time-consuming process of gradual masking warmup during pre-training. As a result, this can be the most efficient and effective approach in practice, which also shares a similar principle as finetuning from RosettaFold in RFDiffusion~\citep{watson2023RFdiffusion}.

Although discrete diffusion pre-training from scratch is challenging, we have also explored several ways to improve it. 
% We can also use community available pre-trained Masked-LMs such as ESM2~\citep{lin2022esmfold} as our first-stage model.
We are also curious about the performance of the vanilla masking warmup strategy and would like to see if it can lead to a better pre-trained DPLM. Besides, inspired by your questions, the training dynamics of discrete diffusion based DPLM is also an interesting and exciting direction deserving further exploration. We leave these as our future work.

% We found that the validation loss of two-stage training from our in-house trained Masked-LM and pre-trained ESM2 is very close, and as shown in \Figref{fig:uncond_sample}G, there is also almost no performance gap in the unconditional sampling.

\subsection{\ARLM baseline}

We pretrain a \ARLM using autoregressive training objective. 
In order to be comparable with \method, the autoregressive language model we trained adopts the same architecture as \method, which is the same architecture as ESM2. 
To be capable of adapting the autoregressive training, we modify the mask matrix of the attention module to causal mask, which guarantees each token can only attend the previous position and keep unseen for future. 
The training objective is next word prediction, and we process the input sequence with teacher forcing for efficient parallel training. 
During decoding, we start with \metric{<bos>} token, sample one token each timestep from left to right, and the sampled token in the current timestep will be concatenated to the end of the sequence, becoming input for next timestep. 
The decoding process terminates until \metric{<eos>} token is sampled. Because we can not know when to obtain the \metric{<eos>} token in advance, we can not decide the length of sampled sequence. 
We attempt to force the sampling length by modifying the sampling probability: the probability of \metric{<eos>} is 1 when and only when the sequence length is up to the predefined length, while 0 in all the previous timesteps. 
However, we observe this will decline the quality of sampled sequence significantly.

%\subsection{Novelty}
\subsection{A modified unconditional sampling strategy}

The sampling algorithm proposed in the \citet{zheng2023reparameterized} is to unmask positions with top-k prediction score (log-probability) predicted by $p_{\theta}(\xt{0}|\xt{t})$, and mask all the rest position in each denoising step. 
However, we find that if we use this sampling algorithm to sample sequence unconditionally, the sampled sequence will collapse to trivial pattern, such as repeating with a single amino acid.
We suggest this is because, without any additional conditions, the model initially tends to give a higher prediction score to the amino acids that appear frequently in the training set.
Subsequently, based on these high-frequency amino acid tokens, the model will continue to sample the same tokens beside these tokens with high confidence. 
The other amino acid can also be sampled, but possibly with a lower prediction score, thereby leading to be dropped according to the top-k sampling algorithm.
Then, this amino acid will spread throughout the entire sequence like a virus, forming a sequence composed entirely of the same amino acids.

In response, we impose a slight disturbance during sampling, utilizing the Gumbel-Max trick. 
The Gumbel-Max trick is a procedure for drawing a sample from a categorical distribution using Gumbel-distributed random variables. Let's assume we have a discrete random variable $X$ with distribution $p_\theta(\bm{x} = i) = p_i$ for $i=1,\ldots,K$. Now, consider the variables $g_i = -\log{(-\log{U_i}})$ where $U_i$ is a variable uniformly distributed on $(0,1]$. The $g_i$ are random variables following a Gumbel distribution. The key to the Gumbel-Max trick is this relationship:
\begin{align}
i^* = \argmax_{i}  \{ \Tilde{p}_i \}, ~\text{where}~ \Tilde{p} \propto \exp{g_i + \log {p_i}}
\end{align}
This operation provides a sample from the discrete distribution $p_\theta(\bm{x}=i)$. In other words, the category corresponding to the maximum value is the results of sampling.
But in the other hand, the maximum value, \ie $g_i + \log p_i$, is not equal to the original log-probability, which is actually the prediction score in our sampling algorithm.
Therefore, the Gumbel-Max trick helps us sample an amino acid with a slightly modified prediction score while maintaining the original distribution.
As a result, the previously dominant amino acid with the highest prediction score may be discarded, and a variety of other amino acids may be retained, thereby avoiding falling into a trivial pattern such as repeating with a single amino acid. We find that this technique can significantly reduce the number of trivial cases and further improve the diversity.

% \subsection{Analysis of Timesteps}
% TODO

% \subsection{Secondary Structure Analysis}
% Analyze the secondary structure distribution between EvoDiff, UniRef and \method. 
% The secondary structure distribution of \method is similar to UniRef.
% Meanwhile, we find that the proportion of the sheet structure of \method is higher than UniRef and EvoDiff.
% The amino acids of a sheet structure is spatially close while far away in the sequence, so the sheet structure is relatively hard to model due to the long distance dependence. 
% Therefore, we suggest that it illustrates \method has a good ability in the long distance modeling, leading to better performance on the various application, such as long protein sampling.
% We also investigate the secondary structure distribution across various length proteins. 

% \subsection{Sequence Representation t-SNE}
% TODO

\section{Additional Experimental Results}

\subsection{Sequence-conditional generation: motif-scaffolding}
\begin{table}[t]
\centering
\vspace{-1.5mm}
\caption{Results of the success rate of each problem, the number of the solved problems and the average success rate across 17 motif-scaffolding problems. Here we follow previous work to use OmegaFold as the folding model.}
\label{tab:motif_success}
\vspace{1.5pt}
\resizebox{\linewidth}{!}{%
\begin{tabular}{ccccc}
\toprule
\multirow{2}{*}{} & \multicolumn{2}{c}{{seq-only}} & \multicolumn{2}{c}{{struct-cond.}} \\ 
\cmidrule[0.5pt](lr){2-3}  \cmidrule[0.5pt](lr){4-5}
                  & EvoDiff        & DPLM                 & RFDiffusion        & DPLM   \\
\midrule
1bcf              & 0.39           & \textbf{0.99}        & 1.00                 & 1.00                    \\
1prw              & 0.87           & \textbf{0.96}        & 0.08               & \textbf{0.99}        \\
1qjg              & 0.00              & 0.00                    & 0.00                  & 0.00                    \\
1ycr              & 0.13           & \textbf{0.52}        & 0.74               & \textbf{0.78}        \\
2kl8              & 0.03              & \textbf{0.05}        & 0.88               & 0.05                 \\
3ixt              & 0.26           & 0.20                  & 0.25               & \textbf{0.33}        \\
4jhw              & 0.00              & 0.00                    & 0.00                  & 0.00                    \\
4zyp              & 0.00              & \textbf{0.01}        & 0.40                & 0.01                 \\
5ius              & 0.00              & \textbf{0.10}         & 0.02               & \textbf{0.10}         \\
5tpn              & 0.00              & 0.00                    & 0.61               & 0.00                    \\
5trv              & 0.00              & 0.00                    & 0.22               & 0.00                    \\
5wn9              & 0.00              & \textbf{0.01}        & 0.00                  & \textbf{0.01}        \\
5yui              & 0.06           & \textbf{0.42}        & 0.00                  & \textbf{0.63}        \\
6e6r              & 0.16           & \textbf{0.84}        & 0.71               & \textbf{0.84}        \\
6exz              & 0.00              & \textbf{0.01}        & 0.42               & 0.01                 \\
6vw1              & 0.00           & 0.00                    & 0.69               & 0.00                    \\
7mrx              & 0.00              & \textbf{0.59}        & 0.07               & \textbf{0.59}        \\ 
\midrule
pass rate         & 7/17           & \textbf{12/27}       & 13/17              & 12/17                \\
avg. success rate & 0.09           & \textbf{0.27}        & 0.36               & 0.31                 \\ 
\bottomrule
\end{tabular}
}
\vspace{4mm}
\end{table}

The overall motif-scaffolding results are shown in \Tabref{tab:motif_success}.
We sample 100 scaffold sequences for each motif scaffolding case, and compute the success rate according to the standard mentioned in section~\ref{sec:motif}. Furthermore, we also show the pass rate (e.g. the number of solved problems) and the average success rate for all problems. 
We use sequence-only and structure-conditioned sampling paradigms. 
For sequence-only sampling, DPLM generates scaffold according to the motif sequence fragment.
For structure-conditioned sampling, DPLM makes generation by leveraging both sequence and structure information of motif. 
Specifically, as noted in section~\ref{sec:IF}, we utilize the pre-trained GVPTransformerEncoder and structural adapter to process the motif structure.
DPLM is able to solve 12 of 17 motif scaffolding problems. 
The overall success rate is 0.27 for sequence-only sampling, while 0.31 for structure-conditioned sampling.
It should be noted that not all problems are suitable for using structure information.
We recommend using structure-conditioned sampling for 1YCR, 1PRW, 3IXT and 5YUI, while sequence-only sampling for others.

\input{tables/motif_esmfold}
\paragraph{Evaluation with more advanced folding model.}
Moreover, we also investigate evaluation with other structure prediction models, such as ESMFold~\cite{lin2022esmfold}. 
Results are shown in \Tabref{tab:motif_esmfold}, we consider the Alpha Carbon~(CA) pLDDT score predicted by ESMFold as the overall pLDDT score of the amino acid. 
We observe that ESMFold judges more strictly than OmegaFold. 
When we evaluate scaffold by ESMFold, there is a slight decline in the overall pass rate and average success rate, compared with the evaluation of OmegaFold.

% \paragraph{Analysis}
% The detailed analysis unveiled a common biological property among the motifs observed in these two cases. Specifically, the motif sequence displayed a remarkable level of evolutionary conservation, playing pivotal roles in binding critical signal passengers (1prw: calmodulin EF hand for calcium binding and 5yui: carbonic anhydrase II for CO2 binding). Notably, the motif structures predominantly comprised flexible loops. Conversely, 5TPN, 6VW1, and 2KL8, which exhibited a distinct advantage in motif scaffolding as indicated by the RFdiffusion algorithm, featured rigid helical structures that lacked functional evolutionary conservations. This intriguing phenomenon suggests that DPLM holds great promise as a superior method for constructing structurally flexible yet evolutionarily conserved functional motif scaffolding.

% \begin{figure}[h]
%     %\vspace{-2mm}
%     \centering
%     \includegraphics[width=1.0\linewidth]{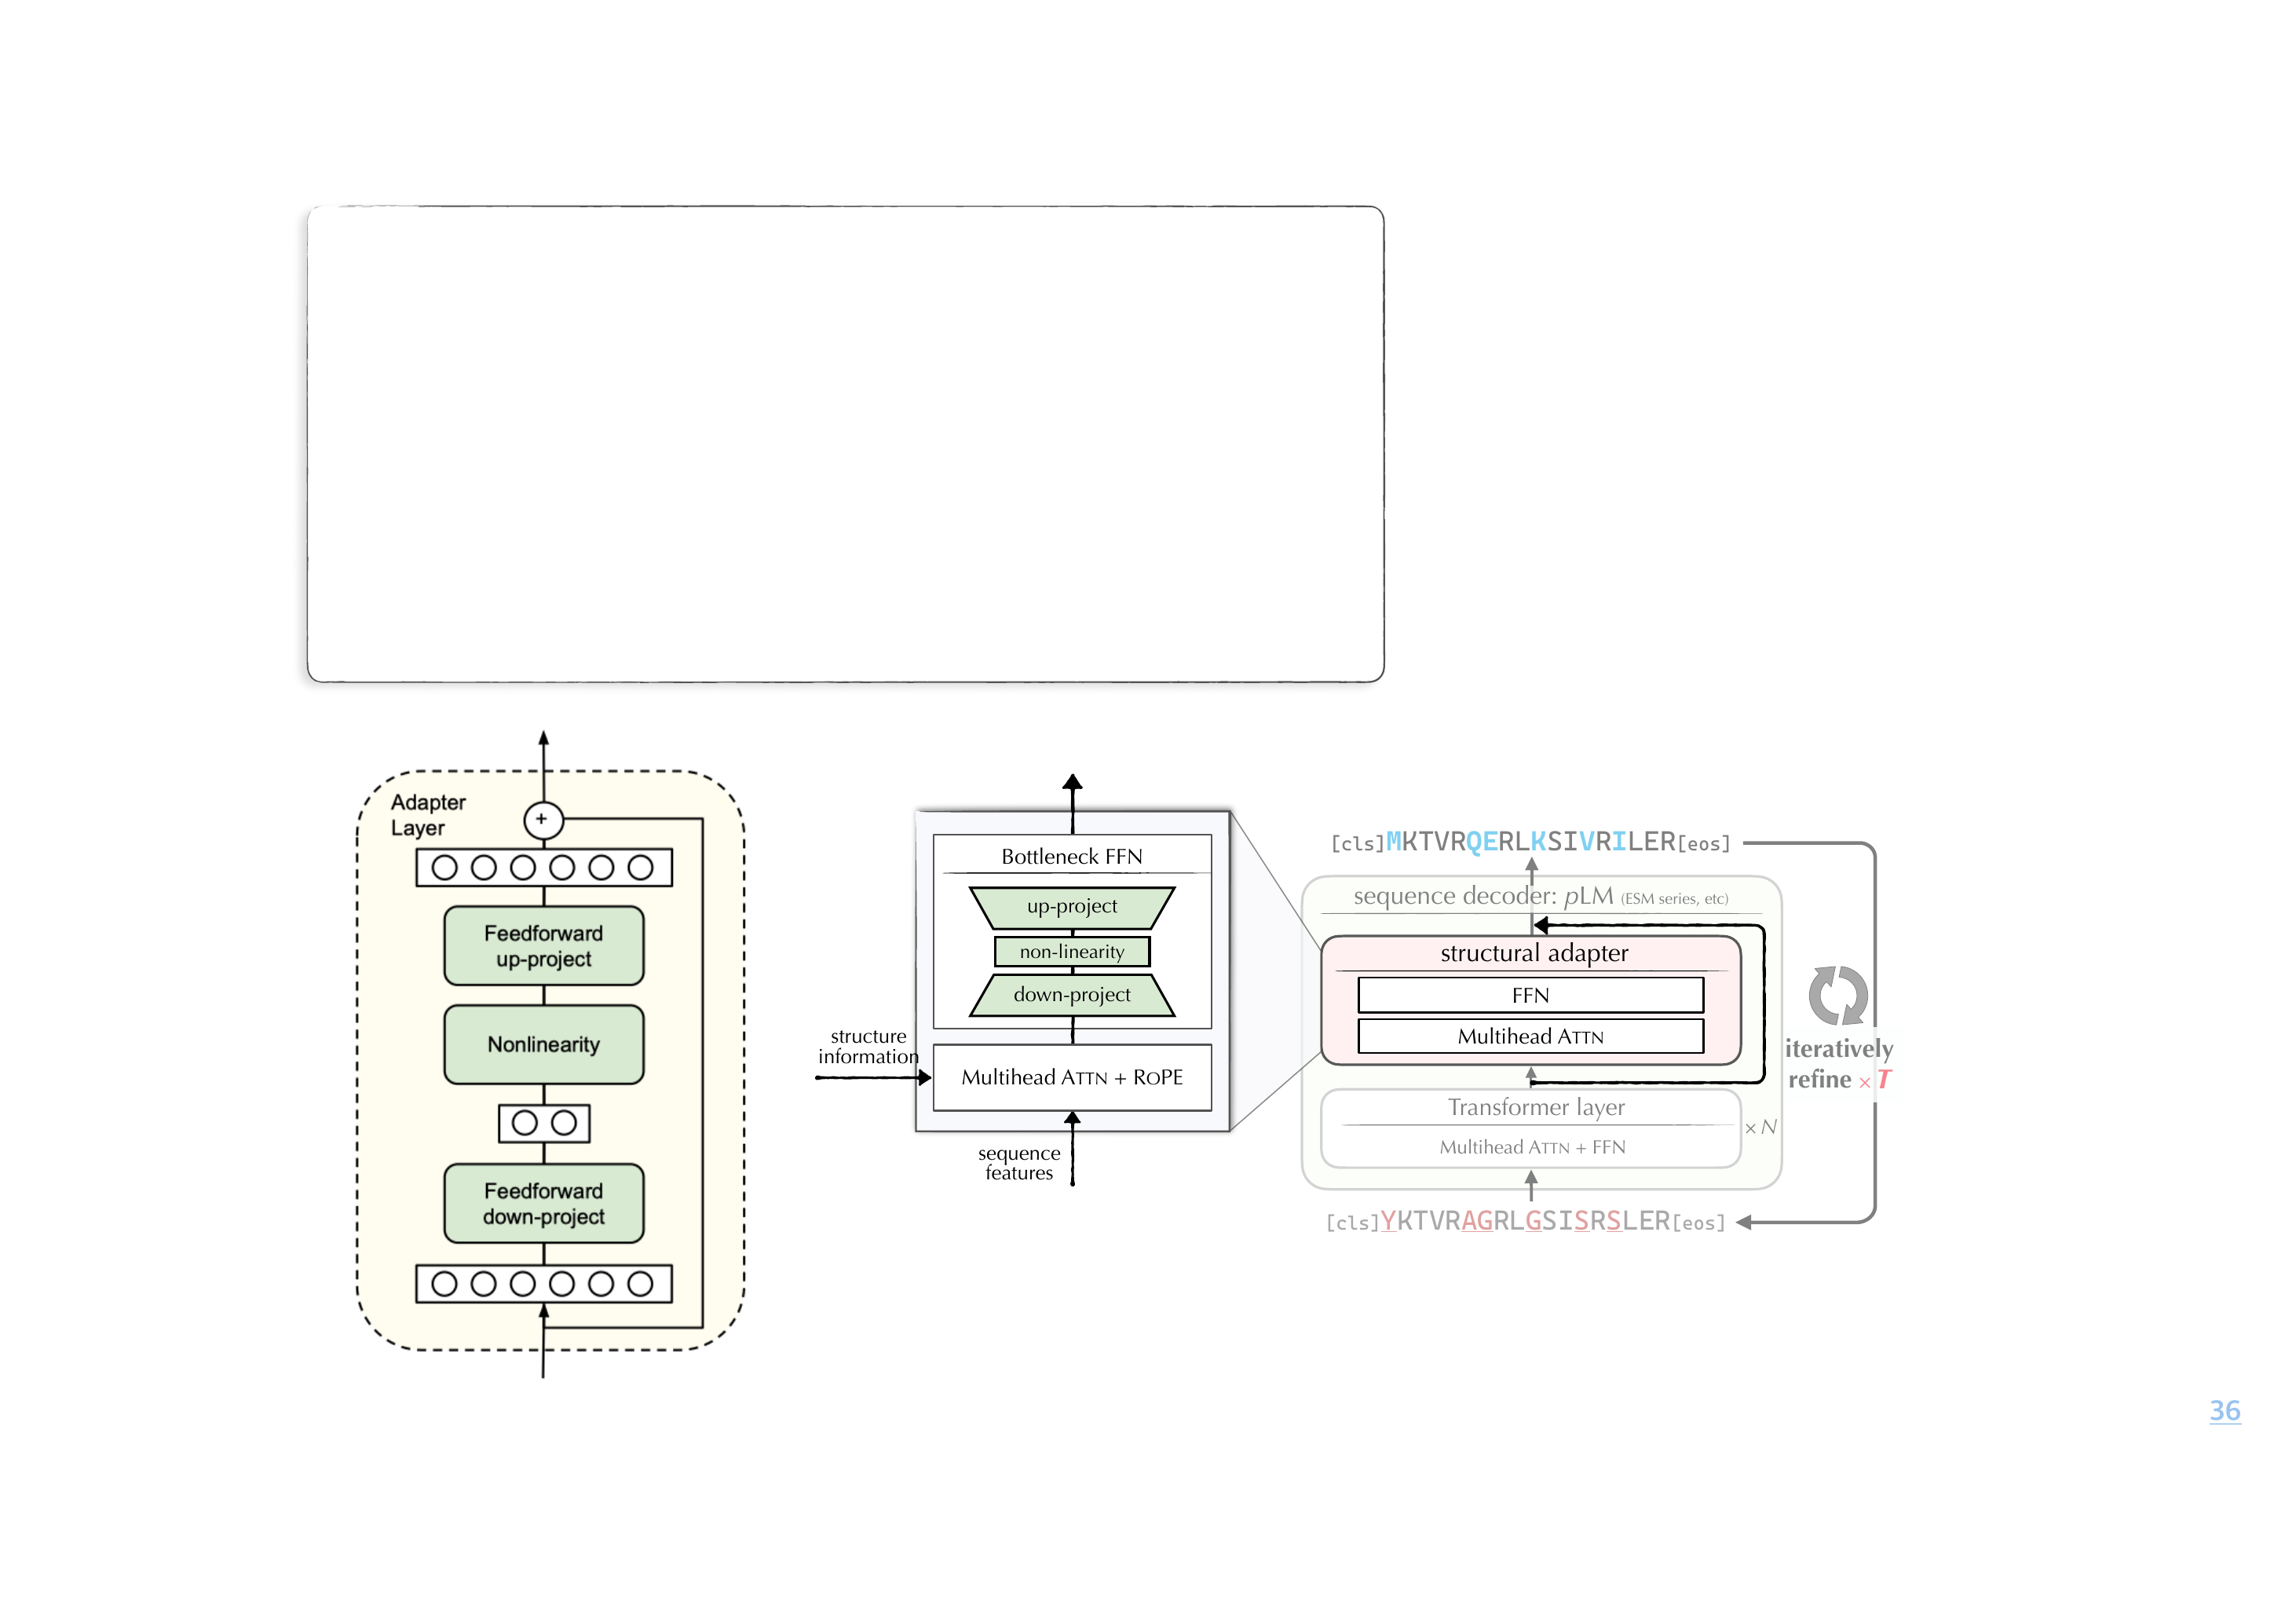}
%     % \vspace{-20pt}
%     \caption{Illustration of the structural adapter that inplanted into \method}
%     \label{fig:adapter}
%     %\vspace{-2mm}
% \end{figure}

\begin{table}[t!]
   \centering
   \small
   \setlength{\tabcolsep}{2pt}
   \vspace{-2.5mm}
   \caption{ Ablation study on the CATH4.3 benchmark, which w/ draft means that the reverse process is based on the $\xt{t}_{draft}$.}
   
   \label{tab:IF_ablation}

   % \resizebox{\linewidth}{!}{%
   \begin{tabular}{lrccc}
   \toprule
    \multirow{2}{*}{ Models} 
   & \multirow{2}{*}{ Trainable} 
   & \multirow{2}{*}{\metric{AAR}} 
   & \multicolumn{2}{c}{ struct. eval.} \\
    \cmidrule[0.3pt](lr){4-5} & Params. & & \metric{scTM}  & \metric{pLDDT} \\
   \midrule
   % StructGNN &  8.29   &   8.74   &  6.40 &   29.44 &   28.26   &  35.91   \\

  % \cmidrule[0.5pt](lr){2-8}

  %%%%%%%%%%%%%%%%%%%%%%%%%%
   % \multirowcell{3}
   \textsc{LM-Design} (\textit{w/} draft)           &  6.3M/650M  & 56.49 &  0.85 & 74.89  \\
  %%%%%%%%%%%%%%% OURS %%%%%%%%%%%%%%%%%%%
  \cmidrule[0.5pt](lr){1-5}
    \method                                                &  6.3M/650M   & 55.75   &  0.83  & 73.72  \\ 
   \chl \method (\textit{w/} draft)                                               & \chl 6.3M/650M   &\chl \textbf{56.61}   & \chl \textbf{0.86}  &\chl \textbf{76.78}  \\ 
  
\bottomrule
\end{tabular}
% }
   \vspace{4mm}
\end{table}

\subsection{Structure-conditional generation: inverse folding}
\paragraph{Model architecture.}
\method only takes amino acid tokens as input, instead of structure formats such as 3D coordinates.
Therefore, in order to endow \method with structural awareness, we follow \textsc{LM-Design}~\citep{zheng2023structure} and place a structural adapter after the last layer of \method, which can attach the structure information to the original output probability. 
The overall architecture of the structural adapter is constituted by three components, \ie, a structure encoder, a \pLM as sequence decoder, and a structural adapter that bridges both. 
We can utilize an arbitrary pretrained structure encoder to process the 3D coordinates and provide structure information for \method.
For \pLMs as the sequence decoder side, we primarily used the \method, with its pretrained model weights. 
The structural adapter composes a multi-head attention that queries structure information from the structure encoder, followed by a \textit{bottleneck} feedforward network (FFN) to impose non-linearity and abstract features/representations. 
% The bottleneck architecture of the FFN adheres to the best practice from \citet{houlsby2019parameter} and many follow-ups of it.
% Most hidden dimensions of \textsc{Multihead Attn} and FFN are determined by the instance of structure encoder and \pLM we used, while the intermediate dimension of the bottleneck FFN was set to be half of the model dimension. 
\textsc{RoPe}~\citep{su2021rope} was used the supplement multi-head attention for better modeling of positional information.
In all our experiments, only one structural adapter was placed after the last layer of \method, following~\citet{zheng2023structure}.

\paragraph{Training and inference details.}
During training, we freeze the parameters of the structure encoder and \method, only optimizing the structural adapter with the simplified discrete diffusion objective~\citep{zheng2023reparameterized}. 
However, we find that there is an exposure bias problem here: \method learns the reverse denoising process based on the ground truth context, \ie $\xt{t}$, which is obtained by adding noise on the ground truth sequence, \ie $\xt{0}$.
During inference, \method has to denoise given the context predicted, which is not always right, leading to training-inference inconsistency.
Therefore, we slightly modify the training objective in \Eqref{eq:reparam_obj}.
Specifically, we obtain $\xt{t}$ by adding noise on the draft sequence generated by the pretrained structure encoder, rather than the ground truth $\xt{0}$, which we refer to as $\xt{t}_{draft}$.
Then \method will learn the reverse process that reconstructs the $\xt{0}$ given the $\xt{t}_{draft}$, as shown in \Eqref{eq:IF_obj}.
Since the draft sequence is available both in training and inference time, the issue of exposure bias is mitigated.
We find this technique can further boost the performance of \method in the inverse folding task, as illustrated in the Tab.~\ref{tab:IF_ablation}

\begin{align}
\mathcal{J}_t 
 = \mathbb{E}_{q(\xt{0})} \bigg[\lambda^{(t)}  \sum_{1 \leq i \leq L} b_i(t) \cdot \log p_{\theta}(\xt{0}_i|\xt{t}_{\textrm{draft}})\bigg], 
\label{eq:IF_obj}
\end{align}

At inference time, we follow the \method generative process, except that we obtain protein sequence via greedy deterministic decoding, instead of random sampling from the distribution.
Besides, considering that we have had an unconditional model, i.e. the \method itself, and a conditional model, \ie, the \method with structural adapter, we can also seamlessly utilize the classifier-free guidance paradigm during inference.

% \section{Antibody task}

\subsection{Classifier-free guidance}
\label{sec:classifier-free}
Classifier-free guidance~\citep{ho2021classifierfree} has been shown as an effective way to enhance conditional diffusion models.
Likewise, for \method, we can derive an implicit classifier using the Bayes rule
\begin{align}
q(\bm{y} | \xt{t-1}) & = q(\bm{y} | \xt{t-1}, \xt{t}) \nonumber \\
& = \frac{q( \xt{t-1} | \xt{t}, \bm{y}) }{q(\xt{t-1} | \xt{t})}q(\bm{y}|\xt{t}). \nonumber
\end{align}
If we already have an unconditional model $p_\theta(\xt{t-1}| \xt{t})$ and a conditional model $p_\theta(\xt{t-1} | \xt{t}, \bm{y})$ as the estimates, then by substituting this implicit classifier into Eq.~\ref{eq:classifier-guidance}, we can obtain
\begin{align}
    \xt{t-1} & \sim p_\theta(\xt{t-1}| \xt{t}) p_\phi(\bm{y} | \xt{t-1})^{\eta} \nonumber \\
    & \propto p_\theta(\xt{t-1} | \xt{t}) \big( \frac{p_\theta( \xt{t-1} | \xt{t}, \bm{y})}{p_\theta(\xt{t-1} | \xt{t})}\big)^{\eta} \nonumber \\
    & =  p_\theta( \xt{t-1} | \xt{t}, \bm{y})^{\eta} \cdot  p_\theta(\xt{t-1}|\xt{t})^{(1-\eta)},\nonumber
\end{align}
wherein when $\eta = 1$, it is equivalent to sampling from the original conditional \method without guidance, whereas $\eta > 1$, we not only prioritize the conditional model to contribute more but also discourage the samples from moving away from the unconditional distribution. 
In other words, it reduces the chance of generating samples that do not use conditioning information, in favor of the samples that explicitly do.

Note that when we use adapter tuning to adapt \method for conditional generation, we only finetune the newly-added parameters, which means that we can already access both the unconditional model (original \method) and conditional model (the adapter-tuned model) simultaneously for free. 
As demonstrated in \Figref{fig:classifier_free} on structure-conditioned sequence generation, we can find that \method as a diffusion model can benefit from classifier-free guidance, improving its conditional generation immediately. 

\begin{figure}[h!]
    \centering
    \vspace{2mm}
    \includegraphics[width=0.9\linewidth]{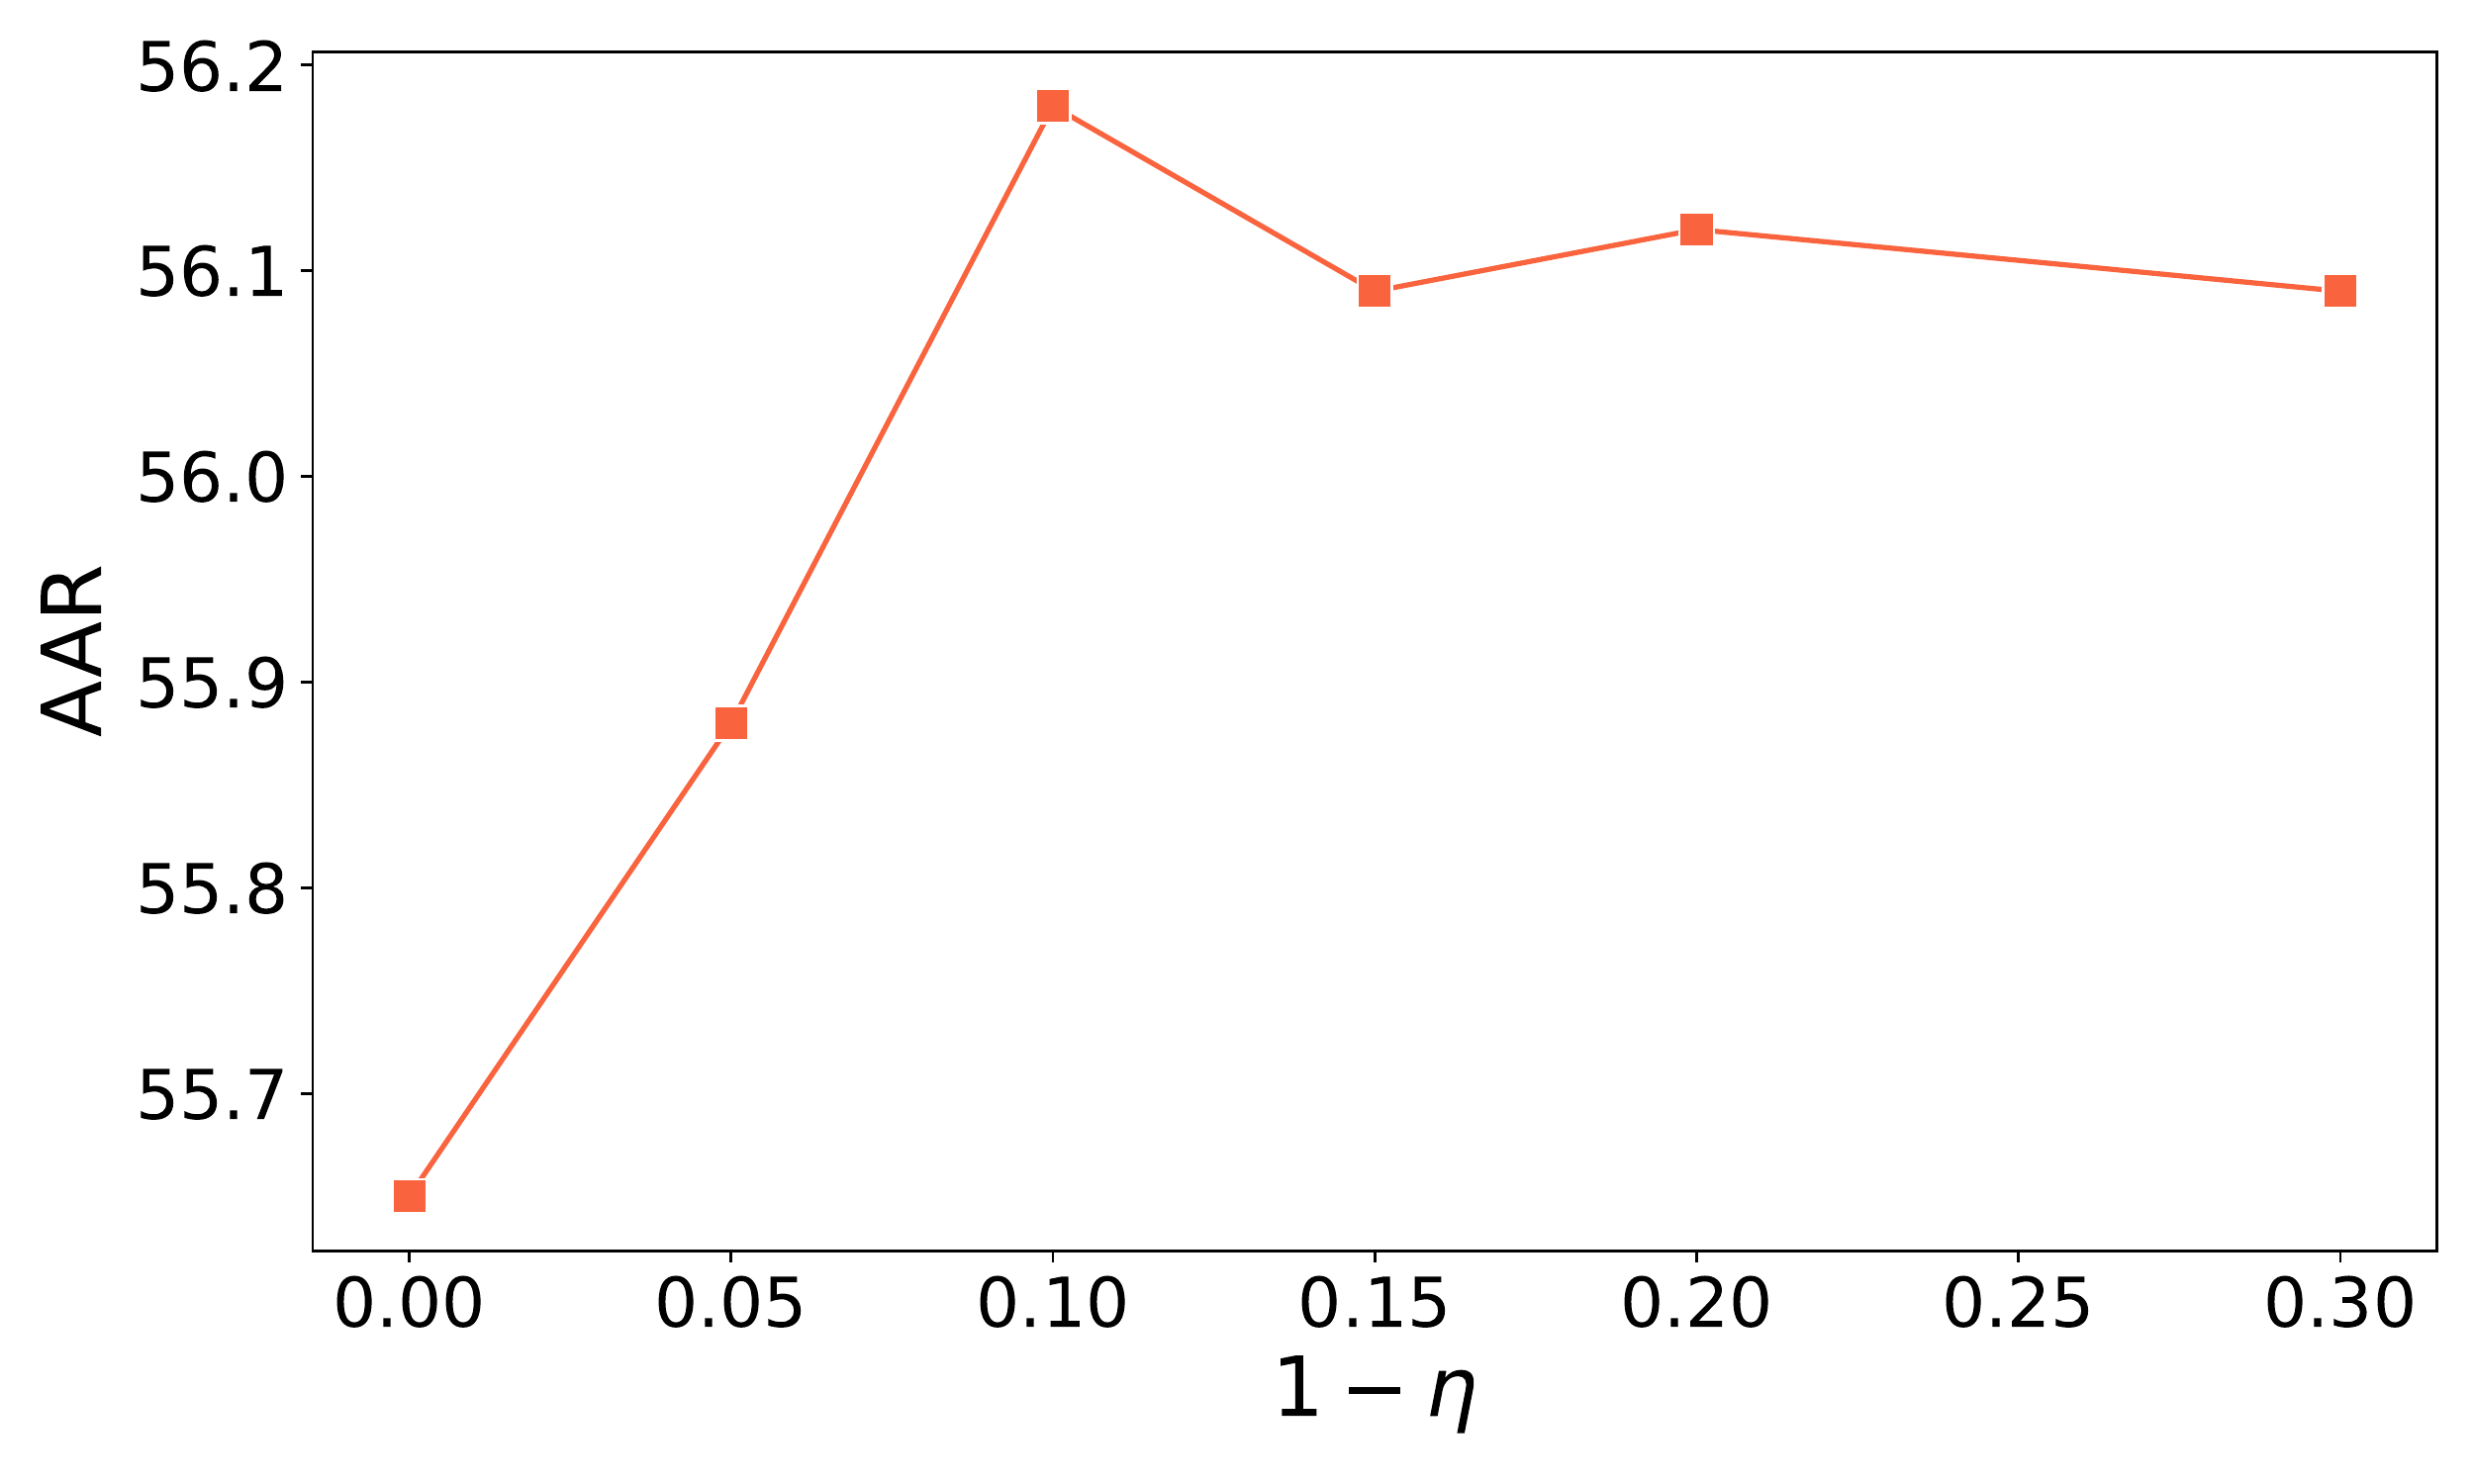}
    \vspace{-4mm}
    \caption{Classifier-free guidance enhances structure-conditioned sequence generation (inverse folding).} 
    \label{fig:classifier_free}
    \vspace{4mm} 
\end{figure}

\section{Related Work}
\label{sec:related}

\subsection{Language Models}
% Language models learn with self-supervised objectives.
% This enables 
The dominant paradigm of language models is autoregressive language models, which breaks down the mutual distribution over the tokens of a sequence into conditional probabilities via the chain rule ${p(\bm{x}^{[1:N]})=\prod_{i=1}^N p(x^{[i]}|\bm{x}^{[1:i-1]})}$ and generates tokens by ancestral sampling from left to right~\citep{bengio2000neural,sutskever2014sequence,vaswani2017attention}.
Recently, researchers propose the non-autoregressive language models as an alternative~\citep{gu2018non}. 
These models do not need to obey the left to right generation order~\citep{qian2022diff,huang2022PDAT} and demonstrate competitive or superior performance compared to their autoregressive counterpart across a wide range of domains including languages~\citep{qian2021volctrans,huang2022PDAT,qian2022diff,huang2022PDAT,zheng2023reparameterized}, speeches~\citep{kim2021conditional}, proteins~\citep{zheng2023structure}, and molecules~\citep{hoogeboom2022equivariant}.
Among the numerous non-autoregressive language models, diffusion language models~\citep{li2022diffusionlm,gong2022diffuseq,zheng2023reparameterized} have emerged as a solid and promising framework.
Pretraining language models on a massive scale of unlabeled data markedly improves their downstream task performance~\citep{word2vec,elmo,radford2018gpt,devlin2019bert}.
As data volume and model sizes scale up, the training loss of language models predictably declines~\citep{kaplan2020scaling,hoffmann2022training,muennighoff2023scaling}, and enhancing downstream task performance even without specific tuning~\citep{gpt2}.
GPT3~\citep{brown2020gpt3} is a significant point in the journey, taking model sizes to 175B parameters, proposing in-context learning to bolster language models' competence in solving certain tasks with only a handful of demonstrations.
Furthermore, \citet{wei2021flanv1,t0,ouyang2022instructgpt} introduce instruction tuning, finetuning pretrained language models on series of tasks described via instructions, which elicits the instruction following ability of models and significantly enhances their zero-shot performance on unseen tasks.
More impressively, sufficiently large language models exhibit the emergent abilities such as multi-step reasoning~\citep{kojima2022zeroshotcot,wei2022emergent,wei2022CoT}, which small models do not possess~\citep{fu2023specializing}.
Empowered by large language models, helpful applications such as conversational AI systems\footnote{\url{https://chat.openai.com/}} and autonomous agents\footnote{\url{https://github.com/Significant-Gravitas/Auto-GPT}} have garnered much interest.
Although the most capable models at the moment are restricted in access, open-sourced efforts~\citep{zeng2022glm,touvron2023llama,touvron2023llama2,alpaca,vicuna2023,moss} have largely enhanced the public accessibility of powerful large language models.

\subsection{Protein Language Models}
% A large body of work has focused on modeling the sequences for proteins.
Thanks for the abundance of 1D amino acid sequences, there is growing interest in developing protein LMs at the scale of evolution, such as the series of ESM~\citep{rives2019esm,lin2022esmfold}, TAPE~\citep{rao2019evaluating}, 
ProtTrans~\citep{elnaggar2021prottrans}, PRoBERTa~\citep{nambiar2020transforming}, PMLM~\citep{he2021pre}, 
ProteinLM~\citep{xiao2021modeling}, 
PLUS~\citep{min2021pre}, 
Adversarial Masked LMs~\citep{mcdermott2021adversarial}, 
ProteinBERT~\citep{brandes2022proteinbert}, 
CARP~\citep{yang2022convolutions} in masked language modeling (MLM) paradigm, 
%ProtTrans~\citep{elnaggar2021prottrans}, 
ProtGPT2~\citep{ferruz2022protgpt2} in causal language modeling paradigm, and several others~\citep{melnyk2022reprogramming,madani2021deep,unsal2022learning, nourani2021tripletprot, lu2020self, sturmfels2020profile, strodthoff2020udsmprot}.
These protein language models exhibit remarkable generalization ability on various downstream tasks and be able to capture evolutionary information about secondary and tertiary structures from sequences alone.
Meanwhile, recent study shows these models' potency in revealing protein structures~\citep{lin2022esmfold}, predicting the effect of sequence variation on function~\citep{meier2021language}, antibody infilling~\citep{melnyk2022reprogramming} and many other general purposes~\citep{rives2019esm}.
Simultaneously, \citet{verkuil2022language} demonstrate that the large scale protein LMs can generate \textit{de novo} proteins by generalizing beyond natural proteins, both theoretically and experimentally validating their hypothesis in exhaustive detail, in which \pLMs demonstrate competency in designing protein structure despite being exclusively trained on sequences.

% Recently language models have been proposed for modeling large-scale databases of protein sequences rather than families of related sequences. Examples include (Bepler & Berger, 2019; Alley et al., 2019; Heinzinger et al., 2019; Rao et al., 2019; Madani et al., 2020; Elnaggar et al., 2021; Rives et al., 2021; Rao et al., 2021). Meier et al. (2021) found that the log-likelihoods of large protein language models predict mutational effects. Madani et al. (2021) study an autoregressive sequence model conditioned on functional annotations and show it can generate functional proteins.

%\paragraph{Language Modeling} aims to learn a probabilistic model to describe sequence data $p(\bm{x}^{[1:N]})$ of interest~\citep{shannon1951prediction,Jurafsky2009}. 

\subsection{Diffusion Language Models}
Derived from diffusion models~\citep{sohl2015diffusion}, diffusion language models is a variety of generative model that samples data via an iterative denoising process from noise. They can be divided into continuous~\citep{ho2020ddpm,song2020sde} and discrete~\citep{hoogeboom2021argmax,austin2021structured} categories according to the distribution they model.
Continuous diffusion models make great success in vision~\citep{dhariwal2021diffusionbeatgans,rombach2021highresolution,ho2022imagenvideo}, but they struggle in languages for operating on continuous surrogates of discrete tokens~\citep{li2022diffusionlm,gong2022diffuseq,han2022ssd,cdcd,yuan2022seqdiffuseq,gao2022difformer,ye2023dinoiser,chen2023cheaper,wu2023ar}, which has difficulty bypassing the pitfall of discreteness~\citep{ye2023dinoiser} and still lags behind autoregressive language models.
In contrast, discrete diffusion models, albeit having limited progress in large-scale applications, are innately suited to the data type inherent to languages (\ie, sequences of discrete tokens).
\citet{zheng2023reparameterized} makes commendable strides in discrete diffusion models and enhancing these models to yield comparable performance with autoregressive models on typical language generation benchmarks like machine translation.
Furthermore, as shown by \citet{he2022diffusionbert,zheng2023structure}, there are close relationship between discrete diffusion models and masked language models~(MLM), a widely adopted pretraining paradigm in NLP~\citep{devlin2019bert,liu2019roberta}.
% are closely related to trustworthy masked language models~\citep{ghazvininejad2019mask,he2022diffusionbert} and have 
% Inspired by these discoveries, in this work, we investigate the scalability of diffusion language models to explore their potential further.
Following this line, \citet{ye2023diffusion} propose scaling discrete diffusion LMs with diffusive adaptation, showing strong performance on several conditional text generation tasks, and accessing zero-shot instruction following, few-shot in-context learning and the promise of structured reasoning with instruction tuning.
% The most relevant work to ours is \citet{han2023ssd2} which builds a 13B chat model with continuous simplex-based diffusion language models.
% In contrast, our work focuses on discrete diffusion language models and their general abilities on diverse tasks.

\subsection{Protein Structure Diffusion Models}
Diffusion models have become popular tools in structural biology for protein generation, and their utility has been demonstrated across a range of generative tasks in recent years. \citet{trippe2022diffusion}, along with others, have introduced several diffusion model variants, each with its unique approach. For instance, while some models focus on generating the protein backbone by diffusing over protein coordinates, others, such as those proposed by \citet{wu2022high}, target inter-residue angles. \citet{lin2023generating} and \citet{yim2023framediff} have developed models that handle both the position and orientation of residue frames.
% An integrated approach to both sequence and structure generation has been explored by Lisanza et al. (2023), who presented a method that simultaneously produces sequence and backbone. Anand \& Achim (2022) have expanded on this to include side-chain atoms as well. Additionally, Latent Diffusion Models (LDMs) are gaining traction for various applications, including protein sequence synthesis by Jiang et al. (2023), protein backbone construction by Fu et al. (2023), and 3D molecule generation as demonstrated by Xu et al. (2023).
% All these methods utilize latent diffusion processes, adopting different techniques to construct a continuous latent space that effectively encodes input information. For example, one approach divides the latent space into invariant and equivariant components to represent molecules efficiently. The success of these methods in their respective tasks highlights the growing potential and benefits of applying latent diffusion techniques in the field of generative structural biology.
RFDiffusion~\citep{watson2023RFdiffusion} is a model that assists in designing protein structures for specific functions, such as enzymes. It is versatile in protein design and has been used to create therapeutic proteins, with some designs being confirmed in the laboratory.
% SMCDiff~\citep{trippe2022diffusion} is a model that generates scaffold structures for protein motifs. It predicts backbones and then builds scaffolds, yielding longer and more diverse outcomes compared to older methods.
ProteinSGM~\citep{lee2022proteinsgm} is a model that uses 2D matrices, which represent the distances and angles between protein parts, to create 3D protein structures for novel protein designs.
FoldingDiff~\citep{wu2022protein} is a model that generates protein sequences expected to fold into a specific structure. These sequences are verified with prediction tools, although they have not been experimentally confirmed yet.
Chroma~\citep{ingraham2023chroma} is a model designed for creating large proteins and protein complexes, considering various constraints like distances and symmetry. It transforms a collapsed polymer into protein backbone and sequence more quickly than older methods, thereby allowing for the efficient generation of large structures.

\subsection{Protein Inverse Folding}
The structure-based protein sequence design is typically formulated as a conditional sequence generation problem by deep generative modeling, wherein protein 3D structures are usually depicted as a \textit{k}-NN graph~\citep{ingraham2019generative}.
The protein graph establishes edge features between adjacent residues and encodes residue information as node features, modeled by graph neural networks (GNNs).
GraphTrans~\citep{ingraham2019generative} and GVP~\citep{jing2020gvp} utilizes the graph attention encoder and autoregressive decoder for protein design.
Recently, ProteinMPNN~\citep{dauparas2022proteinmpnn} and PiFold~\citep{gao2022pifold} introduce more complex protein features and expressive GNNs, resulting in significant improvements. 
Furthermore, in addition to the primary generative purpose, this task can also be used as a proxy for protein (structure-aware) representation learning~\citep{yang2022masked}.
A critical and significant challenge herein is the lack of sufficient protein structure data.
To this end, ESM-IF~\citep{hsu2022esmif} alleviate this issue with effective data augmentation by back-translation with AlphaFold 2~\cite{jumper2021AF2}.  , resulting in dramatic improvements. 
On the other hand, \citet{zheng2023structure} demonstrate how to efficiently steering large pretrained protein LMs into a structure-informed sequence generative models in a mask-predict generative manner, attaining state-of-the-art results on single-chain and complex protein benchmark.
Most recently, graph diffusion models have also been studied for inverse folding problem~\citep{yi2023gradeif}.

% \clearpage
\newpage
\clearpage

\onecolumn
\section{Visualization of Unconditional Samples}

\begin{figure*}[h!]
\vspace{10mm}
    \centering
    \includegraphics[width=\linewidth]{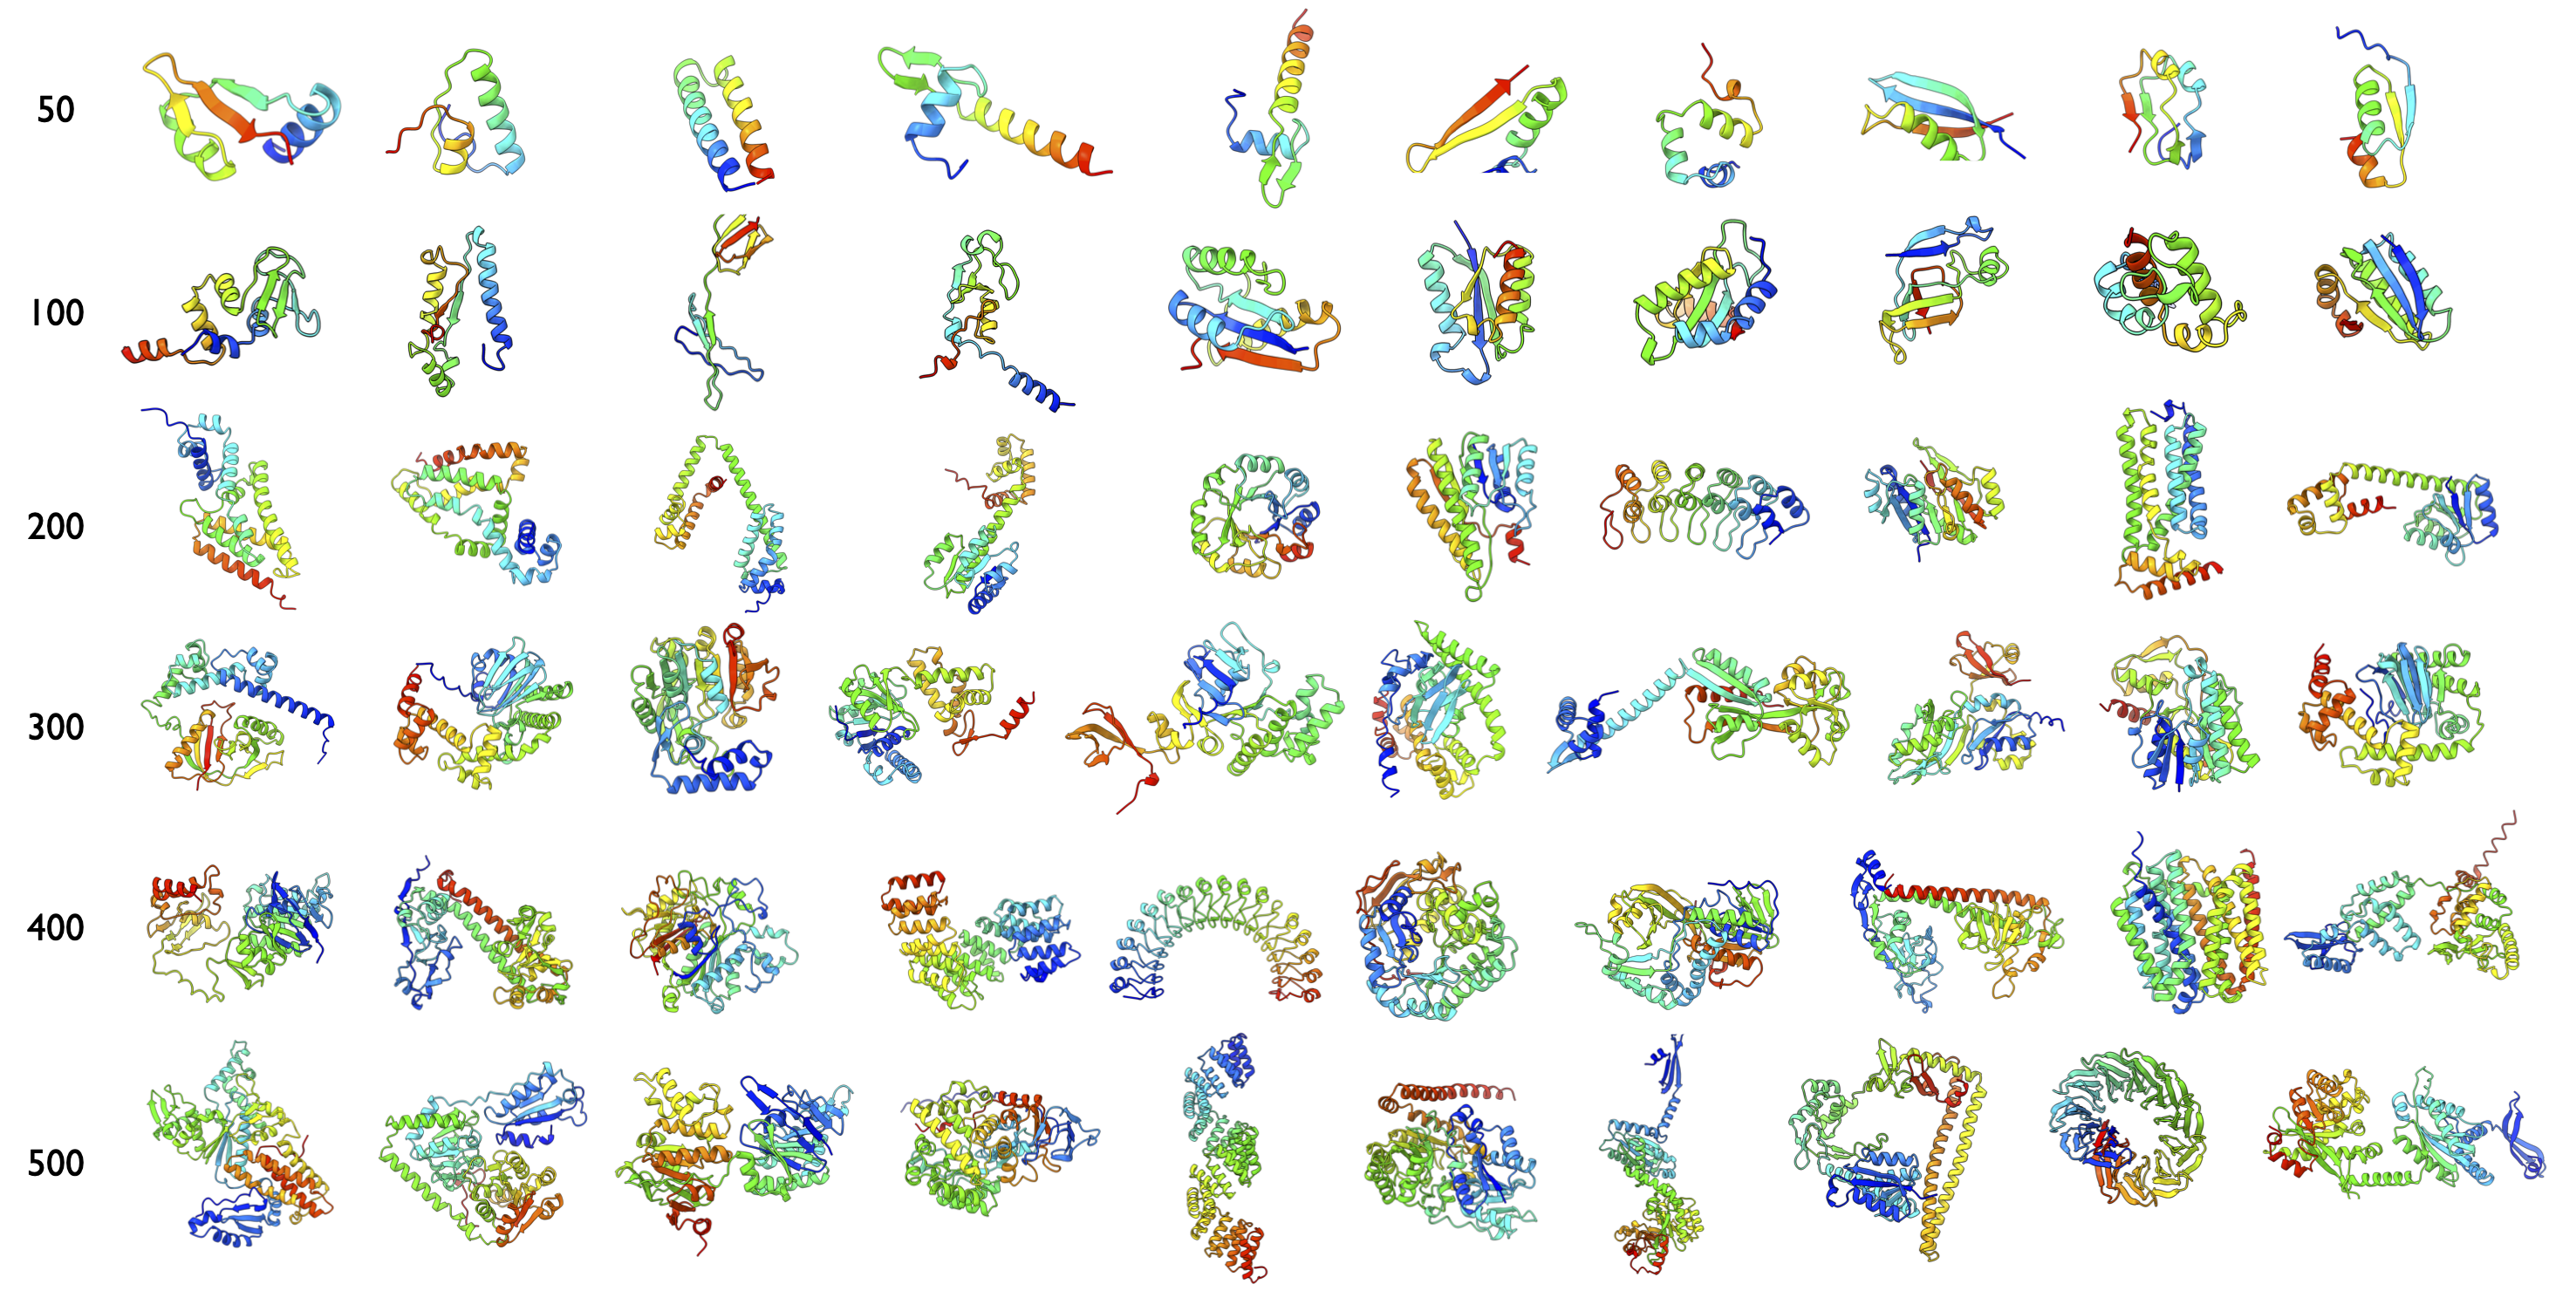}
    \vspace{-4mm}
    \caption{Visualized examples from 50 to 500 in length.} 
    \label{fig:big_pic_100_500}
    \vspace{20mm}
\end{figure*}

\par

\begin{figure*}[h!]
    \centering
    \includegraphics[width=\linewidth]{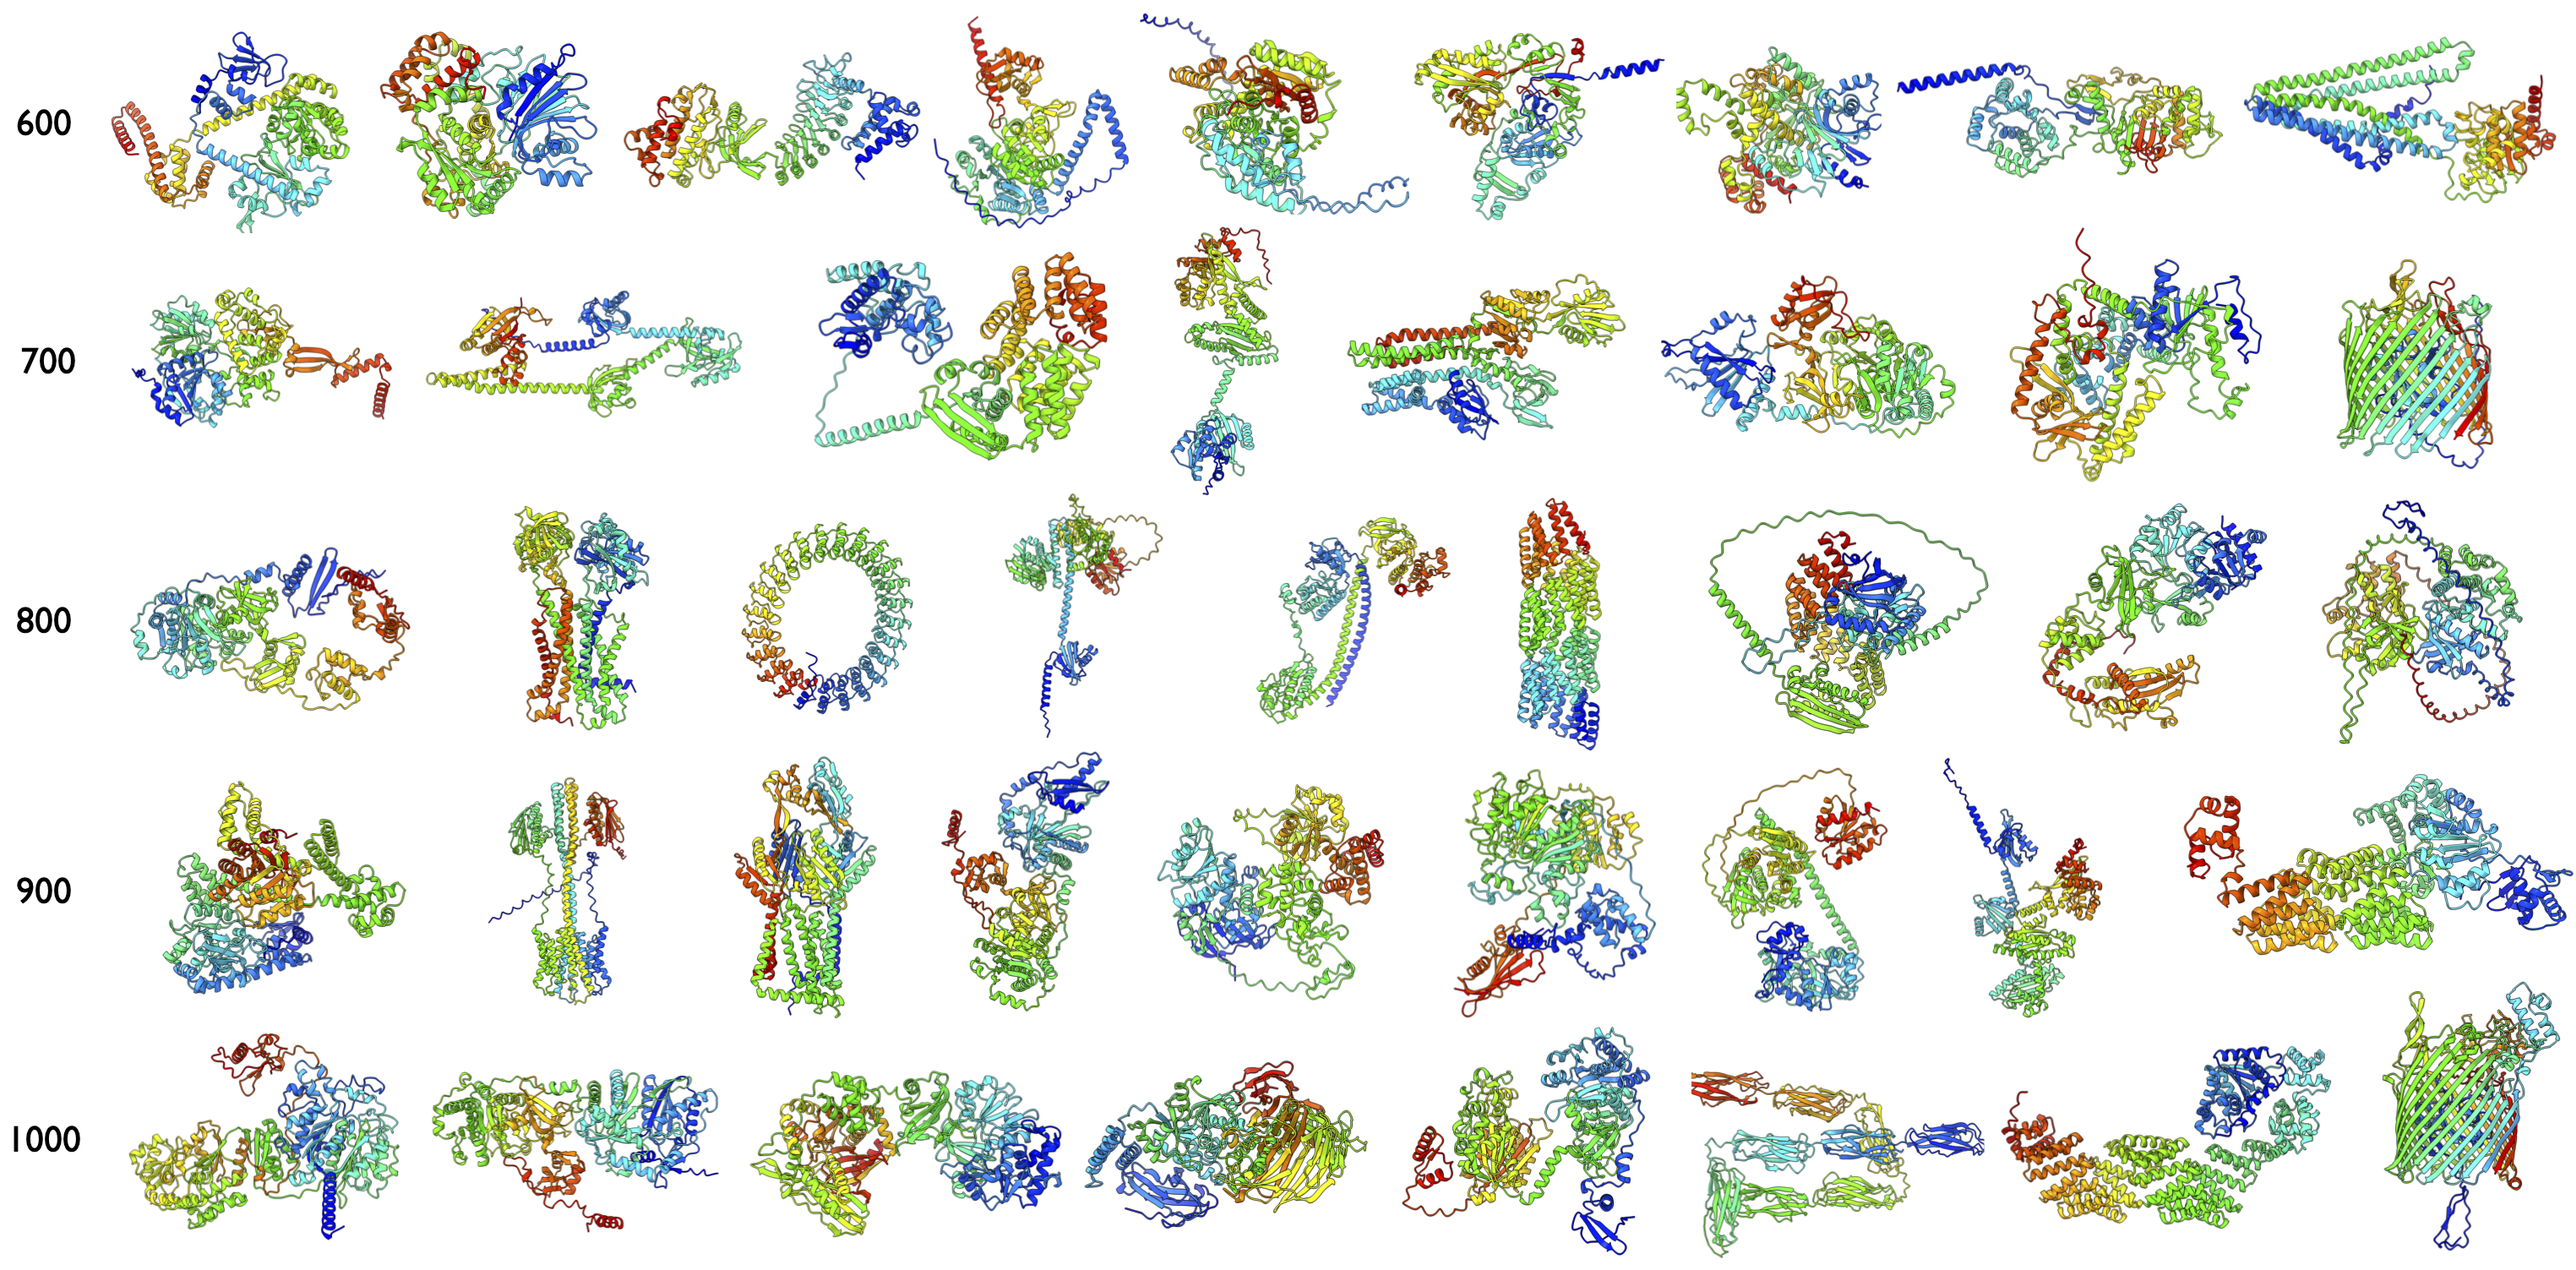}
    \vspace{-4mm}
    \caption{Visualized examples from 600 to 1000 in length.} 
    \label{fig:big_pic_600_1000}
\end{figure*}
